# Supplementary material for: Cascaded Beam Search: Plug-and-Play Terminology-Forcing For Neural Machine Translation
Source: arXiv:2305.14538 source file (2023-05-23)
Supplement: Supplementary file 1 [file appendix.tex]

TODO: add all metrics (copy from sec 2) next to table
